# Supplementary material for: First measurement of neutrino oscillation parameters using neutrinos and antineutrinos by NOvA
Source: arXiv:1906.04907 ancillary file (2019-06-14)
Supplement: Supplementary file 1 [file supplement.pdf]

## First measurement of neutrino oscillation parameters using neutrinos and antineutrinos by NOvA

## Supplemental Figures

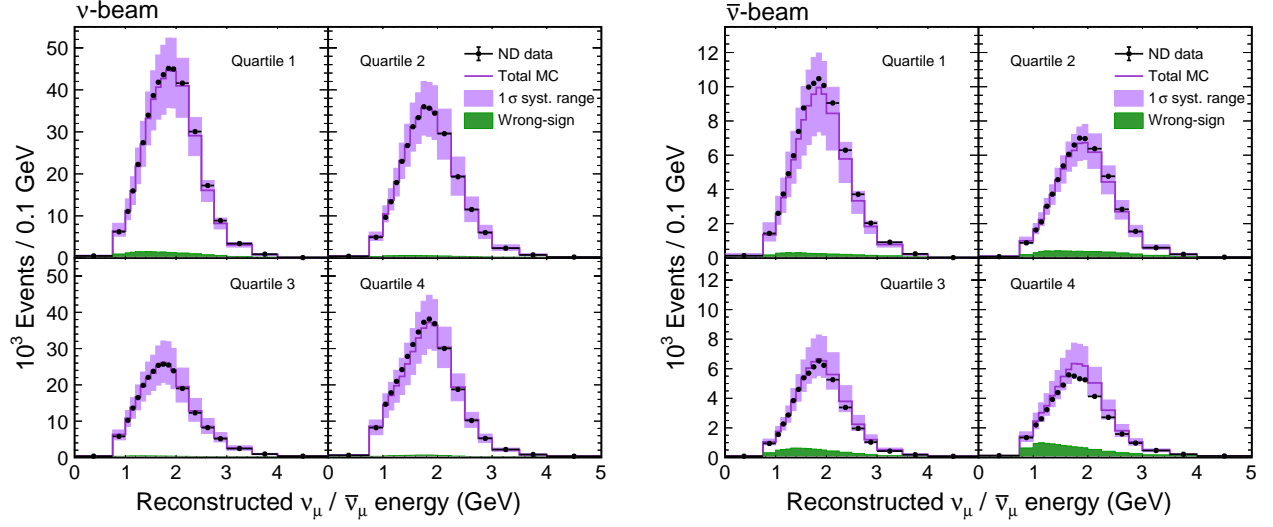

FIG. S1. Reconstructed  $\nu_\mu$  CC energy spectra at the ND shown separately for each quartile of reconstructed hadronic energy fraction, in the neutrino beam on the left and the antineutrino beam on the right. These samples are used to predict the FD  $\nu_\mu$  CC spectra in Fig. S2 below. The spectra are shown with the simulation normalized to the same exposure as the data, and the systematic error band includes all systematic uncertainties.

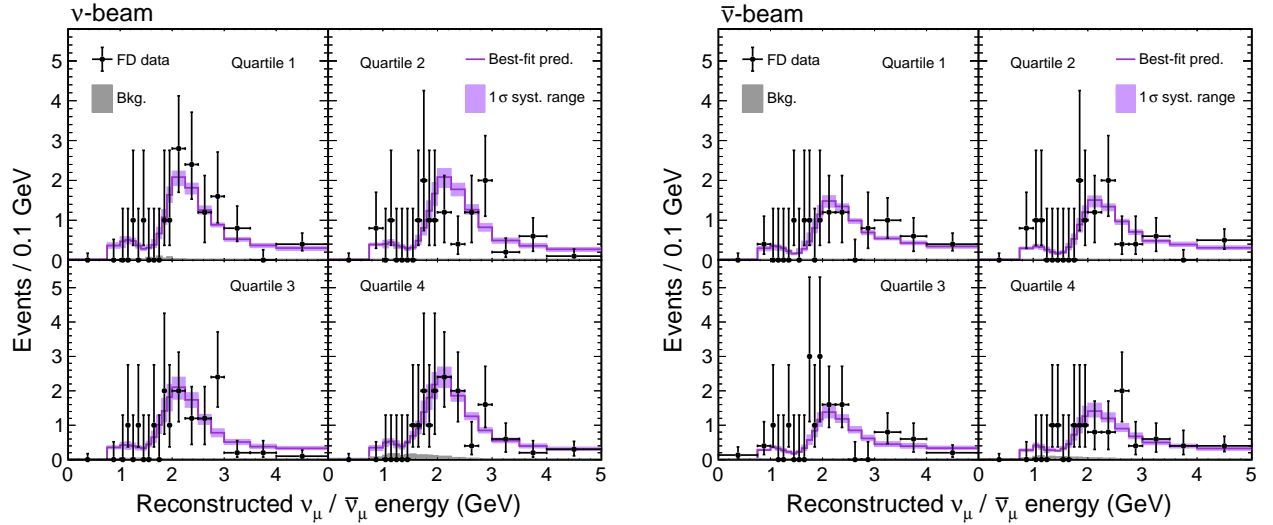

FIG. S2. Reconstructed  $\nu_\mu$  CC energy spectra at the FD shown separately for each quartile of reconstructed hadronic energy fraction, in the neutrino beam on the left and the antineutrino beam on the right. The samples shown here, along with the  $\nu_e$  CC FD samples in Fig. 1, are fit together to extract the oscillation parameters.

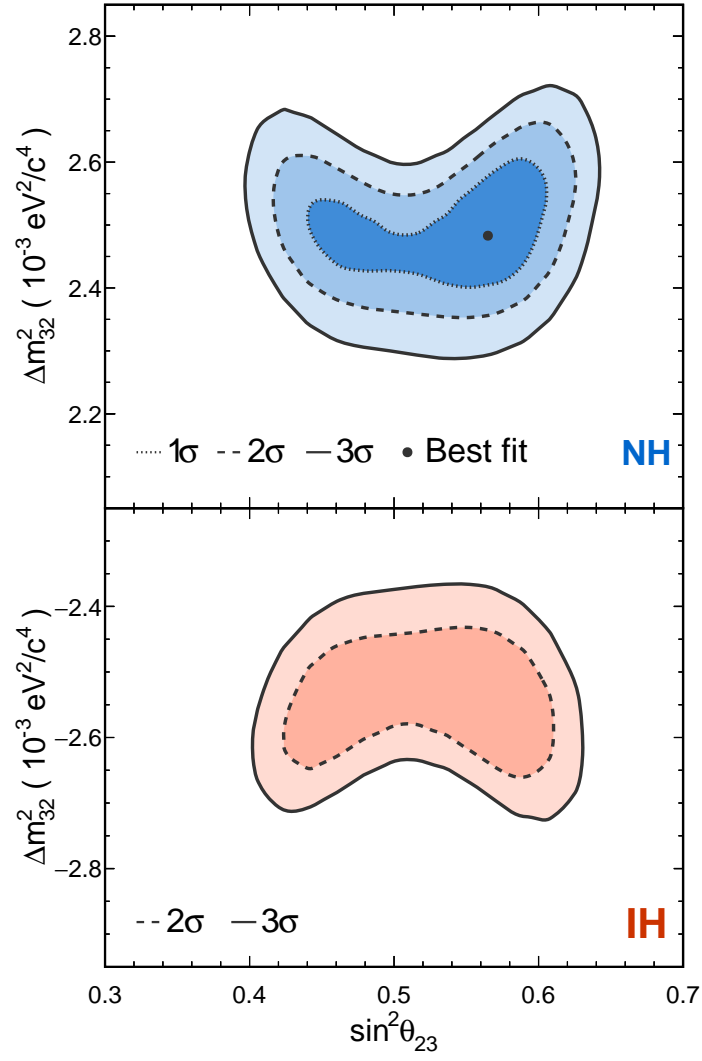

FIG. S3. The  $1\sigma$ ,  $2\sigma$ , and  $3\sigma$  contours in  $\Delta m_{32}^2$  vs.  $\sin^2 \theta_{23}$  in the normal hierarchy (NH, top panel) and inverted hierarchy (IH, bottom panel). The best-fit point is shown by a black marker.

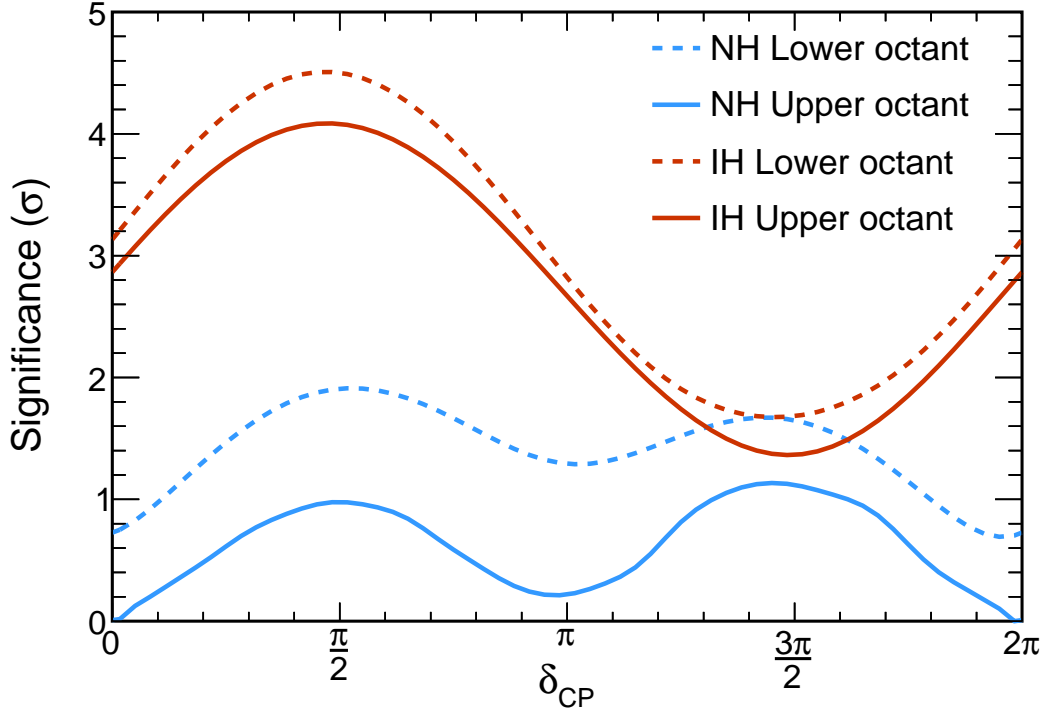

FIG. S4. The projection of the likelihood surface onto the  $\delta_{\text{CP}}$  axis, plotted in terms of significance of rejection of each value of  $\delta_{\text{CP}}$ , under different assumptions of mass hierarchy and the  $\sin^2 \theta_{23}$  octant. Zero significance denotes the best-fit point.

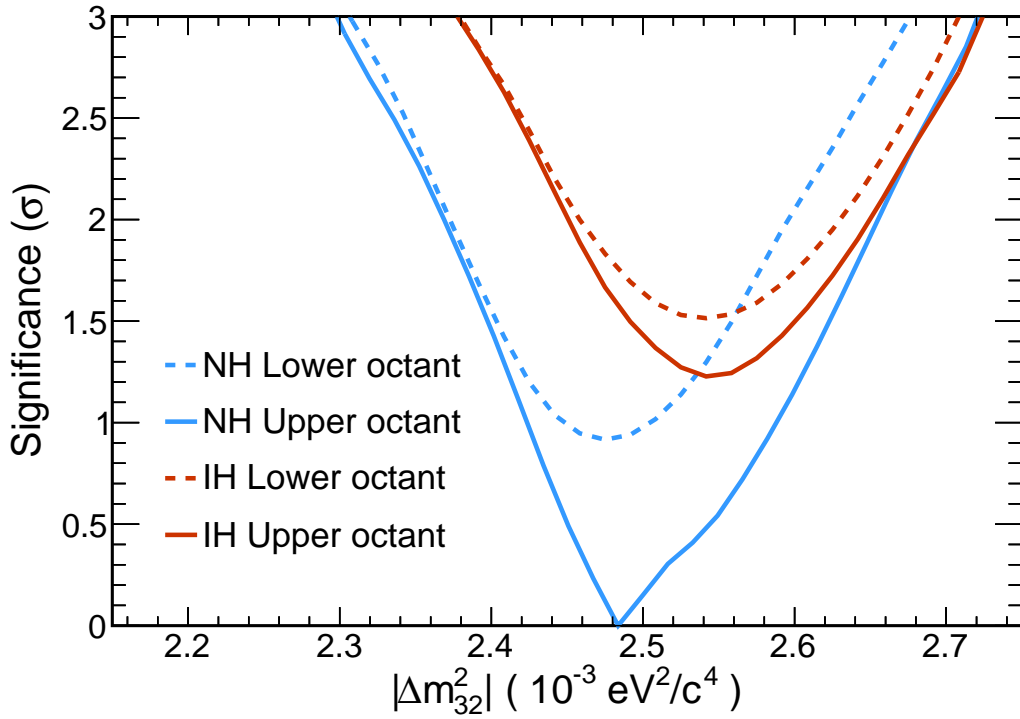

FIG. S5. The projection of the likelihood surface onto the  $\Delta m_{32}^2$  axis, plotted in terms of significance of rejection of each value of  $\Delta m_{32}^2$ , under different assumptions of mass hierarchy and the  $\sin^2 \theta_{23}$  octant. Zero significance denotes the best-fit point.

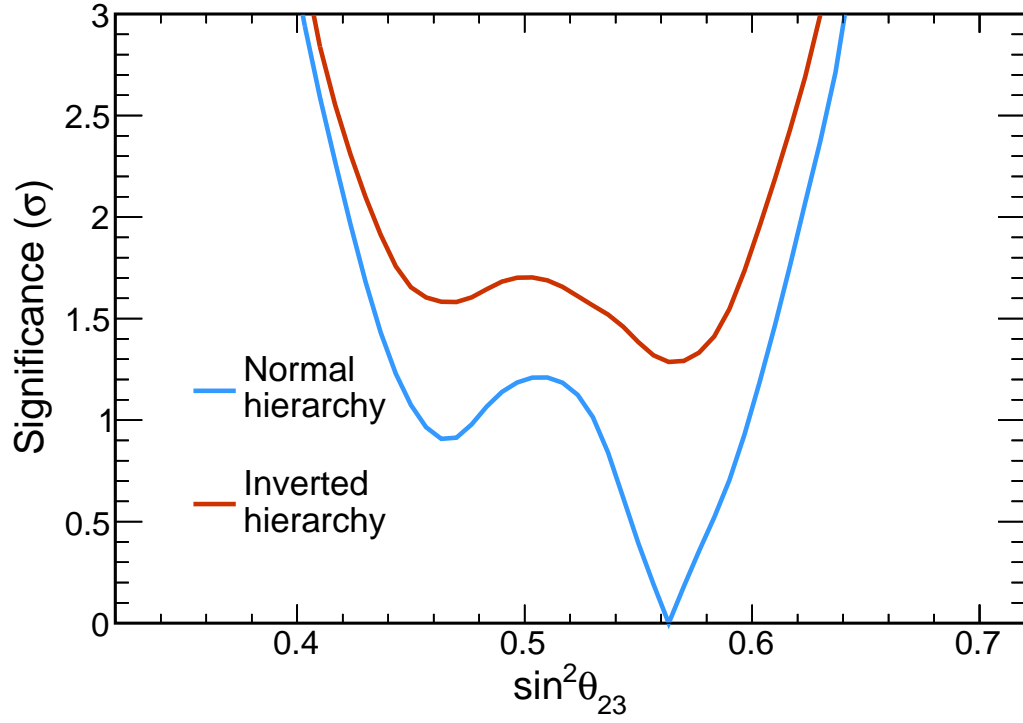

FIG. S6. The projection of the likelihood surface onto the  $\sin^2 \theta_{23}$  axis, plotted in terms of significance of rejection of each value of  $\sin^2 \theta_{23}$ , under different assumptions of mass hierarchy. Zero significance denotes the best-fit point.
